# Supplementary material for: When Automata Meet Streams: Temporal Logic Compilation for Stream-Based Robotics Task and Motion Planning
Source: arXiv:2608.19453 source file (2026-08-19)
Supplement: Supplementary file 1 [file running_example.tex]

% =====================================================================
% running_example.tex
%
% Appendix section for the supplementary material of
% "When Automata Meet Streams: Temporal Logic Compilation for
%  Stream-Based Robotics Task and Motion Planning".
%
% Replaces the inline running example previously in
% supplementary_body.tex. Changes relative to that version:
%   - SAR renamed SAM-PB, TDR renamed SAM-TD, SAM-TD shown first
%   - monitor fluents renamed c1-qk -> M1-qk to match the paper's M_j^k
%   - Valid made nullary, matching the paper (was "(Valid valid-token)")
%   - setup init/goal fixed to use the example's own blocks and fluents
%   - stale references removed (Definition 4, Ex. 2/3/5, DFA image note)
%   - second constraint changed to G(!moved(green)) so it lives in this
%     domain, and the promised multi-constraint continuation is written
%
% Keeps \label{sec-A.1}. Uses the pddl minted environment and booktabs
% from preamble.tex.
%
% Integration: replace the running-example block in
% supplementary_body.tex with \input{running_example}.
% =====================================================================

\section{Running Example: Compiling an Until Constraint}
\label{sec-A.1}

We develop one example end to end: a PDDLStream task, one LTL$_f$ constraint, its automaton, the regressed guards, and the compiled \texttt{pick} schema under both encodings, SAM-TD (\S3.4 of the main paper) and the ablation variant SAM-PB (\S\ref{app:sam-pb}).

\subsubsection{PDDLStream setup}
A robot arm manipulates blocks $\{\mathit{red}, \mathit{blue}, \mathit{green}\}$ on a cluttered table. The domain has three action schemas and four streams:

\begin{pddl}
(:init
    (HandEmpty) (AtConf q-init)
    (AtPose red p-red) (AtPose blue p-blue)
    (AtPose green p-green))
(:goal
    (and (placed red) (placed green)))
\end{pddl}

\begin{pddl}
(:action move
:parameters (?q1 ?t ?q2)
:precondition
    (and (AtConf ?q1) (Motion ?q1 ?t ?q2))
:effect
    (and (AtConf ?q2) (not (AtConf ?q1))))

(:action pick
:parameters (?b ?p ?g ?q)
:precondition
    (and (AtPose ?b ?p) (HandEmpty)
         (Kin ?b ?p ?g ?q) (AtConf ?q))
:effect
    (and (Holding ?b ?g) (moved ?b)
         (not (AtPose ?b ?p)) (not (HandEmpty))
         (not (placed ?b))))

(:action place
:parameters (?b ?p ?g ?q)
:precondition
    (and (Holding ?b ?g) (Kin ?b ?p ?g ?q)
         (AtConf ?q))
:effect
    (and (AtPose ?b ?p) (HandEmpty) (placed ?b)
         (not (Holding ?b ?g))))
\end{pddl}

Streams \texttt{sample-pose}, \texttt{sample-grasp}, \texttt{inverse-kinematics}, and \texttt{plan-motion} certify the static facts \texttt{Pose}, \texttt{Grasp}, \texttt{Kin}, and \texttt{Motion} over continuous objects. The task-level fluents $\mathit{moved}(\cdot)$ and $\mathit{placed}(\cdot)$ record, respectively, that a block has ever been disturbed and that it currently sits at a designated placement; note that \texttt{pick} \emph{adds} $\mathit{moved}(?b)$ and \emph{deletes} $\mathit{placed}(?b)$, so picking a placed block un-places it. The mission goal $G$ requires $\mathit{placed}(\mathit{red}) \wedge \mathit{placed}(\mathit{green})$.

We add a temporal requirement: the blue block must not be disturbed until the red block has been secured at its target. As an LTL$_f$ constraint over $\mathit{AP} = \{\mathit{moved}(\mathit{blue}),\ \mathit{placed}(\mathit{red})\}$:
\[
c_{\mathrm{run}} \;=\; \big(\neg\, \mathit{moved}(\mathit{blue})\big)\ \mathsf{U}\ \mathit{placed}(\mathit{red}).
\]
A second constraint, $c_2 = \mathsf{G}\,\big(\neg\, \mathit{moved}(\mathit{green})\big)$ (``green is never disturbed''), joins at the end of this example to show how multiple constraints share one violation monitor. Until then we develop $c_{\mathrm{run}}$ alone, since its automaton is the smallest one that exercises every rule of the compilation.

\subsubsection{The constraint automaton}
MONA compiles $c_{\mathrm{run}}$ into a three-state DFA $\mathcal{D}_1$ with states $q_1^0$ (initial), $q_1^1$ (accepting), and the sink $q_1^\bot$, whose guarded transition set $\mathcal{T}_1$ (\S3.2) is:
\begin{center}
\small
\begin{tabular}{llll}
\toprule
from & guard $g$ & to & type \\
\midrule
$q_1^0$ & $\mathit{placed}(\mathit{red})$ & $q_1^1$ & forward \\
$q_1^0$ & $\mathit{moved}(\mathit{blue}) \wedge \neg\mathit{placed}(\mathit{red})$ & $q_1^{\bot}$ & sink \\
$q_1^0$ & $\neg\mathit{moved}(\mathit{blue}) \wedge \neg\mathit{placed}(\mathit{red})$ & $q_1^0$ & self \\
$q_1^1$ & $\top$ & $q_1^1$ & self \\
$q_1^{\bot}$ & $\top$ & $q_1^{\bot}$ & self \\
\bottomrule
\end{tabular}
\end{center}
The guards leaving $q_1^0$ partition the alphabet, so exactly one edge fires at each step. Reading the initial valuation, in which neither $\mathit{moved}(\mathit{blue})$ nor $\mathit{placed}(\mathit{red})$ holds, takes the self-loop, so $q_1^{\mathrm{start}} = q_1^0$ (\S3.2).

\subsubsection{Regressing the guards}
We now apply the atomic regression rule of \S3.3 to the two non-self guards:
\begin{align*}
g_{\mathrm{acc}} &= \mathit{placed}(\mathit{red}) \\
g_{\mathrm{sink}} &=
\mathit{moved}(\mathit{blue}) \wedge
\neg \mathit{placed}(\mathit{red}).
\end{align*}
Recall that \texttt{pick} adds $\mathit{moved}(?b)$ and deletes $\mathit{placed}(?b)$, \texttt{place} adds $\mathit{placed}(?b)$, and \texttt{move} touches neither predicate.
\\
\textbf{Regressing through \texttt{pick}:}
For $\mathit{moved}(\mathit{blue})$, \texttt{pick} may add the atom when $?b$ is bound to $\mathit{blue}$:
\[
\mathrm{Reg}_{\texttt{pick}}(\mathit{moved}(\mathit{blue}))
=
\mathsf{Is}\text{-}\mathit{blue}(?b)
\vee
\mathit{moved}(\mathit{blue}).
\]
For $\mathit{placed}(\mathit{red})$, \texttt{pick} may delete the atom when $?b$ is bound to $\mathit{red}$:
\[
\mathrm{Reg}_{\texttt{pick}}(\mathit{placed}(\mathit{red}))
=
\neg \mathsf{Is}\text{-}\mathit{red}(?b)
\wedge
\mathit{placed}(\mathit{red}).
\]
Therefore the sink guard regresses to
\[
\begin{aligned}
\mathrm{Reg}_{\texttt{pick}}(g_{\mathrm{sink}})
={}&
\big(
\mathsf{Is}\text{-}\mathit{blue}(?b)
\vee
\mathit{moved}(\mathit{blue})
\big) \\
&\wedge
\big(
\mathsf{Is}\text{-}\mathit{red}(?b)
\vee
\neg \mathit{placed}(\mathit{red})
\big).
\end{aligned}
\]
Thus, \texttt{pick} enters the sink exactly when it makes blue moved, or blue was already moved, while red is not placed after the action. This condition is derived mechanically from the add/delete effects; it does not require constraint-specific reasoning. \\
\textbf{Regressing through \texttt{place}:}
Here \texttt{place} may add $\mathit{placed}(\mathit{red})$, while $\mathit{moved}(\mathit{blue})$ is unchanged:
\[
\mathrm{Reg}_{\texttt{place}}(g_{\mathrm{acc}})
=
\mathsf{Is}\text{-}\mathit{red}(?b)
\vee
\mathit{placed}(\mathit{red}),
\]
and,
\begin{align*}
    \mathrm{Reg}_{\texttt{place}}(g_{\mathrm{sink}})
    ={}&
    \mathit{moved}(\mathit{blue}) \\
    &\wedge
    \neg\mathsf{Is}\text{-}\mathit{red}(?b)
    \wedge
    \neg\mathit{placed}(\mathit{red}).
\end{align*}
\textbf{Regressing through \texttt{move}:}
The \texttt{move} schema affects neither $\mathit{moved}$ nor $\mathit{placed}$, so the frame case applies to every atom:
\[
\mathrm{Reg}_{\texttt{move}}(g) = g
\]
for both guards. The compiler still emits the corresponding non-self transitions for \texttt{move}; the action is still an LTL$_f$ time step, even though it does not change the guard atoms.

\subsubsection{\texttt{pick} compiled under SAM-TD}
Instantiating the two non-self edges of $\mathcal{T}_1$ with the regressions just derived, SAM-TD (\S3.4) leaves the precondition untouched and injects both edges as conditional effects. The monitor fluent \texttt{(M1-q0)} is the PDDL rendering of $M_1^0$:

\begin{pddl}
(:action pick
 :parameters (?b ?p ?g ?q)
 :precondition
   (and (AtPose ?b ?p) (HandEmpty)
        (Kin ?b ?p ?g ?q) (AtConf ?q))
 :effect
   (and (Holding ?b ?g) (moved ?b)
        (not (AtPose ?b ?p)) (not (HandEmpty))
        (not (placed ?b))
        ;; sink edge q0 -> q_bot: Token Destruction
        (when (and (M1-q0)
                   (or (Is-blue ?b) (moved blue))
                   (or (Is-red ?b)
                       (not (placed red))))
              (not (Valid)))
        ;; forward edge q0 -> q1: lockstep advance
        (when (and (M1-q0) (placed red)
                   (not (Is-red ?b)))
              (and (M1-q1) (not (M1-q0))))))
\end{pddl}

\texttt{place} receives the symmetric injections with its own regressed guards, and \texttt{move} receives the two edges with un-regressed guards. The initial state gains \texttt{(M1-q0)}, \texttt{(Is-blue blue)}, \texttt{(Is-red red)}, and \texttt{(Valid)}; the goal becomes \texttt{(and (placed red) (placed green) (M1-q1) (Valid))}. Observe the concrete effect on search: a \texttt{pick} binding $?b \mapsto \mathit{blue}$ while \texttt{(M1-q0)} holds and red is unplaced remains applicable, but executing it deletes \texttt{(Valid)}. No action re-adds the token, so $h^{\text{FF}}$ assigns the resulting state infinite cost and the branch is discarded before any stream is sampled for it (\S3.5).

\subsubsection{\texttt{pick} compiled under SAM-PB}
Under the ablation variant (\S\ref{app:sam-pb}), the token-destruction effect disappears and the same regressed sink guard reappears, negated, in the precondition:

\begin{pddl}
(:action pick
 :parameters (?b ?p ?g ?q)
 :precondition
   (and (AtPose ?b ?p) (HandEmpty)
        (Kin ?b ?p ?g ?q) (AtConf ?q)
        ;; sink edge q0 -> q_bot, blocked
        (not (and (M1-q0)
                  (or (Is-blue ?b) (moved blue))
                  (or (Is-red ?b)
                      (not (placed red))))))
 :effect
   (and (Holding ?b ?g) (moved ?b)
        (not (AtPose ?b ?p)) (not (HandEmpty))
        (not (placed ?b))
        ;; forward edge q0 -> q1, as in SAM-TD
        (when (and (M1-q0) (placed red)
                   (not (Is-red ?b)))
              (and (M1-q1) (not (M1-q0))))))
\end{pddl}

The initial state gains \texttt{(M1-q0)}, \texttt{(Is-blue blue)}, and \texttt{(Is-red red)}, and the goal becomes \texttt{(and (placed red) (placed green) (M1-q1))}; no token appears anywhere. The same violating binding $?b \mapsto \mathit{blue}$ is now inapplicable outright. The price is representational: the added conjunct is a negation of a conjunction whose regressed guard is disjunctive, and one such block accumulates per sink edge, which is exactly the conjunction of disjunctions that DNF-normalizing translators multiply out into exponentially many operator copies (\S\ref{app:sam-pb}, \S4.3).

\subsubsection{Adding a second constraint}
Finally, compile $c_2 = \mathsf{G}\,(\neg\, \mathit{moved}(\mathit{green}))$ alongside $c_{\mathrm{run}}$. Its DFA $\mathcal{D}_2$ has one accepting state $q_2^0$, with a self-loop while $\neg\mathit{moved}(\mathit{green})$ holds, and a sink edge otherwise, so SAM-TD adds the fluent \texttt{(M2-q0)}, the identity fact \texttt{(Is-green green)}, and, to \texttt{pick}, the single conditional effect
\begin{pddl}
(when (and (M2-q0)
           (or (Is-green ?b) (moved green)))
      (not (Valid)))
\end{pddl}
No second token is introduced: the sink edges of every constraint delete the same \texttt{(Valid)}, which is the compiled state of the one two-state violation monitor tracking all DFAs at once (\S3.5). The goal additionally gains \texttt{(M2-q0)}. Under SAM-PB, by contrast, each further constraint conjoins another negated disjunctive block into every schema's precondition, multiplying the translator's normalization cases as described in \S\ref{app:sam-pb}.
