# Supplementary material for: When Automata Meet Streams: Temporal Logic Compilation for Stream-Based Robotics Task and Motion Planning
Source: arXiv:2608.19453 source file (2026-08-19)
Supplement: Supplementary file 2 [file experiment_1a_constraint_tables.tex]

% Include this file from paper/current_version.tex after issuing \appendix.
\section{Experiment 1: Arbitrary LTL$_f$ Constraint Catalogs}
For each environment, Experiment 1 uses one fixed, task-specific
LTL$_f$ catalog. The five seed values label predetermined orderings of the
same catalog. At level $k$, the planner jointly enforces the first $k$
constraints in the selected ordering. Labels $G_i$, $U_i$, and $F_1$ denote
safety, strong-until precedence, and eventual-completion constraints,
respectively; each catalog table defines the corresponding formula.
\input{appendix/experiment_1a_tabletop_constraints}
\input{appendix/experiment_1a_kitchen_constraints}
\input{appendix/experiment_1a_zonesort_constraints}
