# Supplementary material for: When Automata Meet Streams: Temporal Logic Compilation for Stream-Based Robotics Task and Motion Planning
Source: arXiv:2608.19453 source file (2026-08-19)
Supplement: Supplementary file 5 [file experiment_1a_zonesort_constraints.tex]

% Experiment 1a ZoneSort appendix tables (single-column layout).
% Frozen source:
% experiments/experiment_1/experiment_1a/protocol/
% Requires booktabs and amsmath, both loaded by the main file.

\providecommand{\eoneorder}[1]{%
  \begin{minipage}[t]{\linewidth}\raggedright #1\end{minipage}}
\providecommand{\eonecell}[2]{%
  \begin{minipage}[t]{0.86\columnwidth}\raggedright
    #1\\[0.5pt]{\scriptsize\itshape #2}\end{minipage}}

\begingroup
\renewcommand{\arraystretch}{1.35}
\begin{table}[t]
\centering
\footnotesize
\caption{Experiment 1a ZoneSort constraint catalog ($G$: safety, $U$:
precedence, $F$: completion). The six safety formulas cover
$b_1,\ldots,b_6$; the nine precedence formulas form the complete bipartite
graph $\{b_1,b_2,b_3\}\rightarrow\{b_4,b_5,b_6\}$.}
\label{tab:e1a-zonesort-catalog}
\begin{tabular}{@{}l@{\hspace{8pt}}l@{}}
\toprule
ID & LTL$_f$ formula and interpretation \\
\midrule
$G_1$ & \eonecell{$\mathsf{G}\bigl(\neg\mathit{InDanger}(b_1)\bigr)$}%
  {Block $b_1$ uses the certified route.} \\
$G_2$ & \eonecell{$\mathsf{G}\bigl(\neg\mathit{InDanger}(b_2)\bigr)$}%
  {Block $b_2$ uses the certified route.} \\
$G_3$ & \eonecell{$\mathsf{G}\bigl(\neg\mathit{InDanger}(b_3)\bigr)$}%
  {Block $b_3$ uses the certified route.} \\
$G_4$ & \eonecell{$\mathsf{G}\bigl(\neg\mathit{InDanger}(b_4)\bigr)$}%
  {Block $b_4$ uses the certified route.} \\
$G_5$ & \eonecell{$\mathsf{G}\bigl(\neg\mathit{InDanger}(b_5)\bigr)$}%
  {Block $b_5$ uses the certified route.} \\
$G_6$ & \eonecell{$\mathsf{G}\bigl(\neg\mathit{InDanger}(b_6)\bigr)$}%
  {Block $b_6$ uses the certified route.} \\
$U_1$ & \eonecell{$\neg\mathit{moved}(b_4)\ \mathsf{U}\ \mathit{sorted}(b_1)$}%
  {Sort $b_1$ before moving $b_4$.} \\
$U_2$ & \eonecell{$\neg\mathit{moved}(b_5)\ \mathsf{U}\ \mathit{sorted}(b_1)$}%
  {Sort $b_1$ before moving $b_5$.} \\
$U_3$ & \eonecell{$\neg\mathit{moved}(b_6)\ \mathsf{U}\ \mathit{sorted}(b_1)$}%
  {Sort $b_1$ before moving $b_6$.} \\
$U_4$ & \eonecell{$\neg\mathit{moved}(b_4)\ \mathsf{U}\ \mathit{sorted}(b_2)$}%
  {Sort $b_2$ before moving $b_4$.} \\
$U_5$ & \eonecell{$\neg\mathit{moved}(b_5)\ \mathsf{U}\ \mathit{sorted}(b_2)$}%
  {Sort $b_2$ before moving $b_5$.} \\
$U_6$ & \eonecell{$\neg\mathit{moved}(b_6)\ \mathsf{U}\ \mathit{sorted}(b_2)$}%
  {Sort $b_2$ before moving $b_6$.} \\
$U_7$ & \eonecell{$\neg\mathit{moved}(b_4)\ \mathsf{U}\ \mathit{sorted}(b_3)$}%
  {Sort $b_3$ before moving $b_4$.} \\
$U_8$ & \eonecell{$\neg\mathit{moved}(b_5)\ \mathsf{U}\ \mathit{sorted}(b_3)$}%
  {Sort $b_3$ before moving $b_5$.} \\
$U_9$ & \eonecell{$\neg\mathit{moved}(b_6)\ \mathsf{U}\ \mathit{sorted}(b_3)$}%
  {Sort $b_3$ before moving $b_6$.} \\
$F_1$ & \eonecell{$\mathsf{F}\bigl(\bigwedge_{i=1}^{6}\mathit{sorted}(b_i)\bigr)$}%
  {Eventually sort all six blocks.} \\
\bottomrule
\end{tabular}
\end{table}
\endgroup

\begingroup
\renewcommand{\arraystretch}{1.15}
\begin{table}[t]
\centering
\footnotesize
\caption{Five frozen ZoneSort prefix orders. Entries are read from left to
right: a run at level $k$ jointly enforces the first $k$ constraints.
The seed values are stable pool labels, not run-time shuffle instructions.}
\label{tab:e1a-zonesort-seeds}
\begin{tabular}{@{}c@{\hspace{8pt}}p{0.82\columnwidth}@{}}
\toprule
Seed & Ordered constraints \\
\midrule
11 & \eoneorder{$F_1$, $U_6$, $U_8$, $G_5$, $U_2$, $U_4$, $G_3$,
  $U_1$, $G_1$, $U_9$, $G_6$, $U_7$, $G_2$, $G_4$, $U_3$, $U_5$} \\
17 & \eoneorder{$U_5$, $U_8$, $G_2$, $F_1$, $U_1$, $G_6$, $U_9$,
  $U_3$, $G_3$, $U_7$, $U_2$, $G_4$, $G_1$, $U_6$, $U_4$, $G_5$} \\
23 & \eoneorder{$U_2$, $U_6$, $G_1$, $G_2$, $U_4$, $U_1$, $F_1$,
  $U_3$, $G_5$, $U_7$, $U_9$, $G_6$, $G_4$, $G_3$, $U_5$, $U_8$} \\
31 & \eoneorder{$U_8$, $G_6$, $U_1$, $U_9$, $U_6$, $G_3$, $U_4$,
  $G_4$, $G_2$, $F_1$, $U_5$, $U_7$, $G_1$, $G_5$, $U_2$, $U_3$} \\
47 & \eoneorder{$G_4$, $U_1$, $U_4$, $U_8$, $U_6$, $G_5$, $U_5$,
  $G_1$, $U_2$, $G_3$, $U_3$, $G_6$, $F_1$, $U_7$, $G_2$, $U_9$} \\
\bottomrule
\end{tabular}
\end{table}
\endgroup
