# Supplementary material for: When Automata Meet Streams: Temporal Logic Compilation for Stream-Based Robotics Task and Motion Planning
Source: arXiv:2608.19453 source file (2026-08-19)
Supplement: Supplementary file 6 [file supplementary.tex]

% =====================================================================
% STANDALONE ANONYMOUS TECHNICAL APPENDIX
%
% This file is compiled separately from anonymous_submission.tex.
%
% Build:  pdflatex -shell-escape supplementary
%         bibtex   supplementary
%         pdflatex -shell-escape supplementary
%         pdflatex -shell-escape supplementary
% =====================================================================

\documentclass[letterpaper]{article} % DO NOT CHANGE THIS
\usepackage[submission]{aaai2027}    % Anonymous review mode
\input{preamble}

% Main-paper pointers render as prose because the paper is separate.
\renewcommand{\mainfigref}[1]{the corresponding figure in the main paper}

\begin{document}
\maketitle
\appendix

\input{Supplementary/Sections/instantiation_incompatibility}
\input{Supplementary/Sections/formal_properties_discussion}
\input{Supplementary/Sections/sam_pb}
\input{Supplementary/Sections/adversarial_constraints}
\input{Supplementary/Sections/pddl3_scaling}
\input{Supplementary/Sections/exp1}

\bibliography{aaai2027}
\end{document}
